# Supplementary material for: Proceedings of the 19th International Overture Workshop
Source: arXiv:2110.09371 source file (2021-10-18)
Supplement: Supplementary file 1 [file appendix.tex]

\appendix
\subsubsection*{Appendix:}
Our work in progress (Overture Project) is available at: \url{https://tinyurl.com/VDMIMM}.
